# Supplementary material for: Unsupervised Compositional Concepts Discovery with Text-to-Image Generative Models
Source: arXiv:2306.05357 source file (2023-08-03)
Supplement: Supplementary file 1 [file model.tex]

\centering
\vspace{-25pt}
\includegraphics[width=\linewidth]{supp_figs/imgs/model.pdf}
\vspace{-20pt}
\captionof{figure}{\small{
       \textbf{Our method.} Given a set of unlabeled images, we discover a set of concepts whose composed scores are trained to denoise and reconstruct images.
    }}
\label{fig:supp_model}
\vspace{8pt}
